# Supplementary material for: Aladdin: Zero-Shot Hallucination of Stylized 3D Assets from Abstract Scene Descriptions
Source: arXiv:2306.06212 source file (2023-06-09)
Supplement: Supplementary file 1 [file antichrist_vatican_BASELINE.tex]

\begin{figure*}\centering\includegraphics[width=0.9 \textwidth]{figures_system_outputs/antichrist_vatican_BASELINE.png}\caption{Baseline output for ``antichrist in the bedroom of the pope"}\label{fig:antichrist_vatican_baseline}\end{figure*}
