# Supplementary material for: Aladdin: Zero-Shot Hallucination of Stylized 3D Assets from Abstract Scene Descriptions
Source: arXiv:2306.06212 source file (2023-06-09)
Supplement: Supplementary file 2 [file busy_new_york_street_BASELINE.tex]

\begin{figure*}\centering\includegraphics[width=0.9 \textwidth]{figures_system_outputs/busy_new_york_street_BASELINE.png}\caption{Baseline output for ``a busy street in downtown new york"}\label{fig:busy_new_york_street_baseline}\end{figure*}
