# Supplementary material for: Aladdin: Zero-Shot Hallucination of Stylized 3D Assets from Abstract Scene Descriptions
Source: arXiv:2306.06212 source file (2023-06-09)
Supplement: Supplementary file 4 [file kings_hand_OURS.tex]

\begin{figure*}\centering\includegraphics[width=0.9 \textwidth]{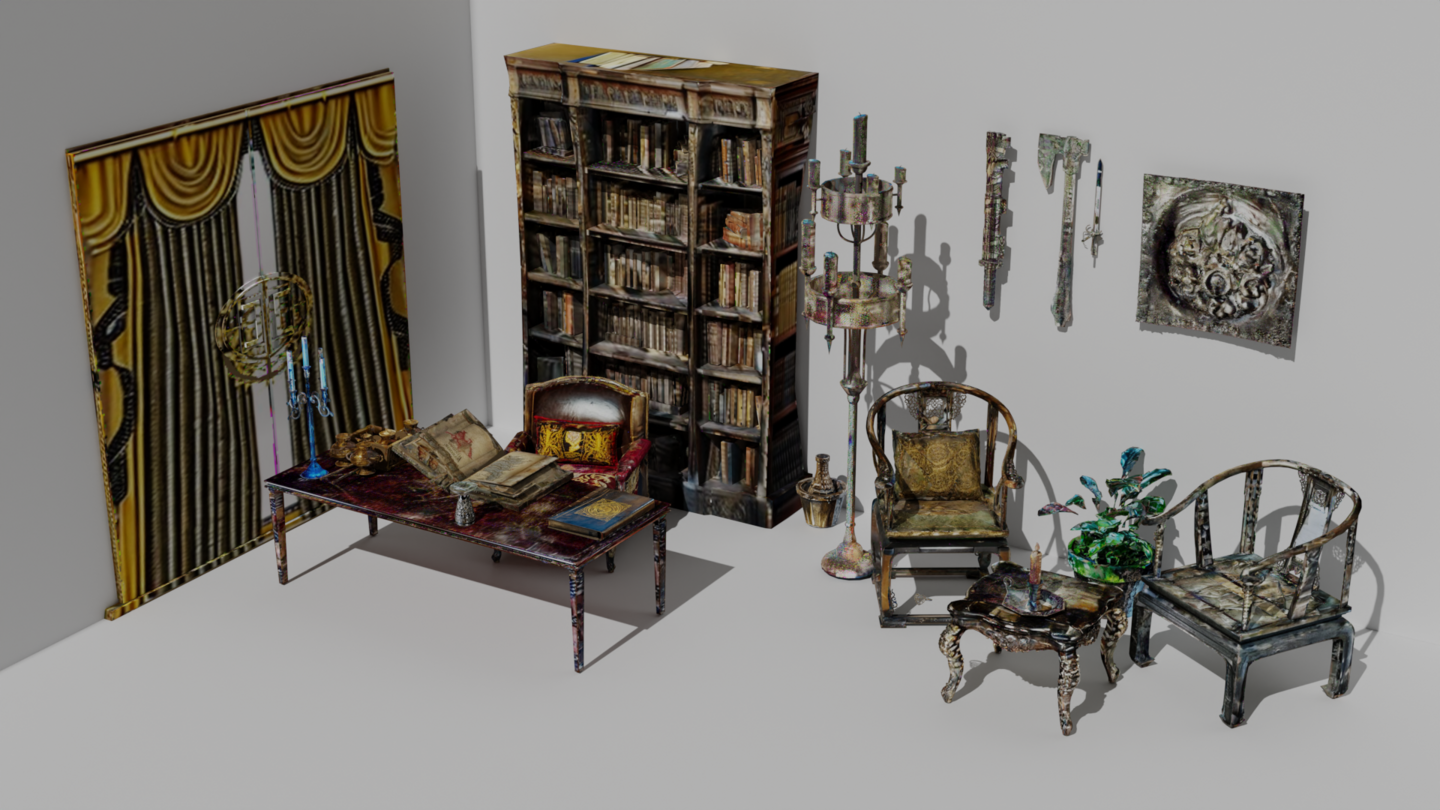}\caption{Our output for ``“Office of King’s Hand in Game of Thrones”"}\label{fig:kings_hand_ours}\end{figure*}
