# Supplementary material for: Aladdin: Zero-Shot Hallucination of Stylized 3D Assets from Abstract Scene Descriptions
Source: arXiv:2306.06212 source file (2023-06-09)
Supplement: Supplementary file 5 [file mad_scientist_restaurant_BASELINE.tex]

\begin{figure*}\centering\includegraphics[width=0.9 \textwidth]{figures_system_outputs/mad_scientist_restaurant_BASELINE.png}\caption{Baseline output for ``a michelin star restaurant opened by a mad scientist"}\label{fig:mad_scientist_restaurant_baseline}\end{figure*}
