# Supplementary material for: Aladdin: Zero-Shot Hallucination of Stylized 3D Assets from Abstract Scene Descriptions
Source: arXiv:2306.06212 source file (2023-06-09)
Supplement: Supplementary file 6 [file north_korean_classroom_BASELINE.tex]

\begin{figure*}\centering\includegraphics[width=0.9 \textwidth]{figures_system_outputs/north_korean_classroom_BASELINE.png}\caption{Baseline output for ``a north korean classroom"}\label{fig:north_korean_classroom_baseline}\end{figure*}
