# Supplementary material for: Aladdin: Zero-Shot Hallucination of Stylized 3D Assets from Abstract Scene Descriptions
Source: arXiv:2306.06212 source file (2023-06-09)
Supplement: Supplementary file 8 [file rustic_backyard_BASELINE.tex]

\begin{figure*}\centering\includegraphics[width=0.9 \textwidth]{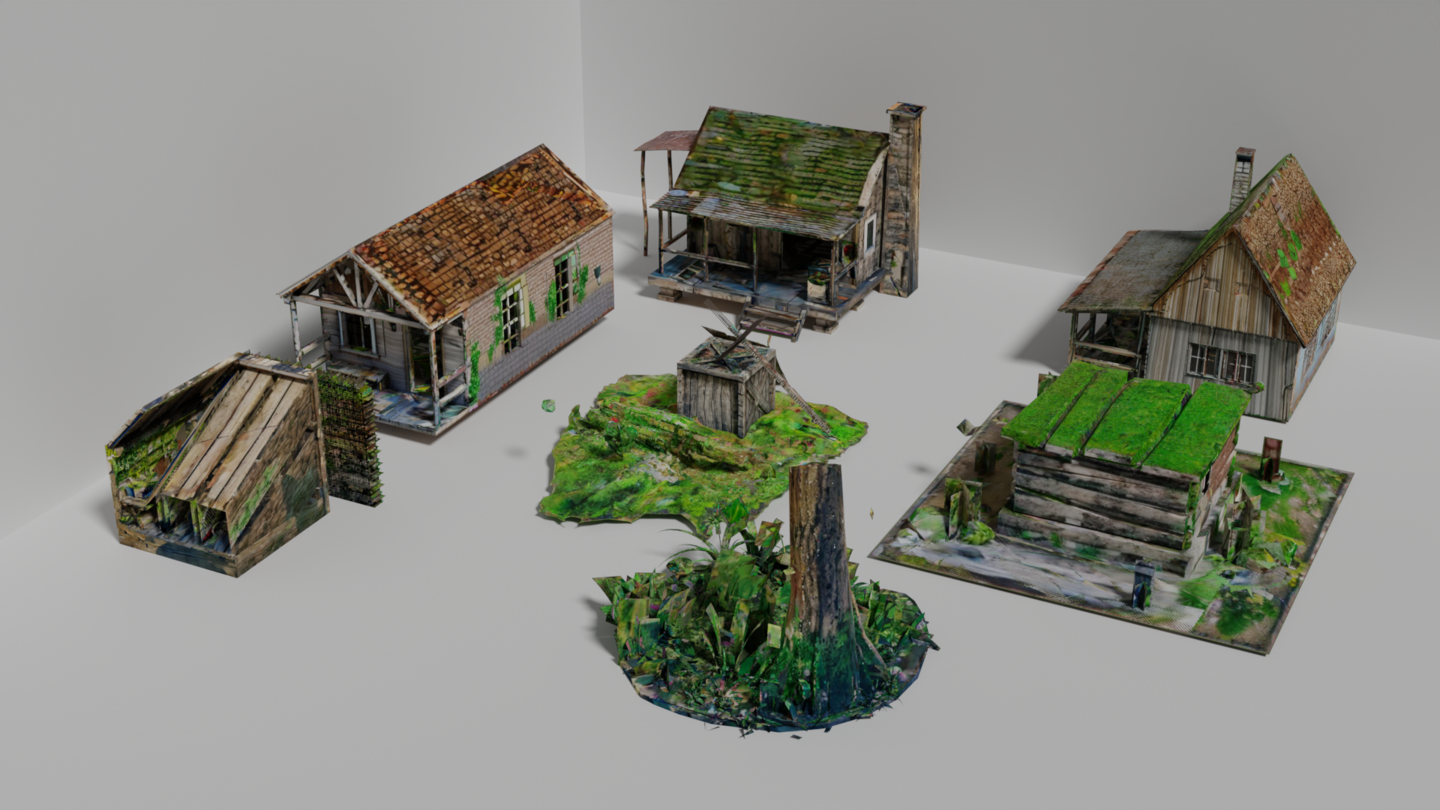}\caption{Baseline output for ``a rustic backyard in the countryside"}\label{fig:rustic_backyard_baseline}\end{figure*}
